# Supplementary material for: Magnetic Levitation Stabilized by Streaming Fluid Flows
Source: arXiv:1805.08608 source file (2018-05-24)
Supplement: Supplementary file 1 [file Supplemental_Baldwin_Magnetic_Levitation_Stabilised_by_Streaming_Fluid_Flows.pdf]

# Magnetic Levitation Stabilized by Streaming Fluid Flows: Supplemental Information

K. A. Baldwin,[1,2] J.-B. de Fouchier,[2] P. S. Atkinson,[2] R. J. A. Hill,[3] M. R. Swift,[3] and D. J. Fairhurst[2]

[1]*Max Planck Institute for Dynamics and Self-Organization, 37077 Göttingen, Germany*
[2]*School of Science and Technology, Nottingham Trent University, Nottingham, NG11 8NS, UK*
[3]*School of Physics and Astronomy, University of Nottingham, Nottingham, NG7 2RD, UK*

(Dated: May 22, 2018)

## EXTENDED METHODS

### Levitation setup

The drive magnet consists of two neodymium disc magnets connected by a brass brass bridge, which were taken from parts of a Stuart SD162 Hotplate Stirrer. The bar was driven to rotate about its centre by a Stuart SS20 mechanical stirrer. An accurate measure of the rotation rate is obtained using an ST-6234B Photo Tachometer, with $\pm 0.3$ rad s$^{-1}$ uncertainty.

Positioned above the rotating magnet is a glass tank, containing a sealed Perspex cylinder, with inner diameter $d = 65$ mm, which contains the fluid under examination and a rare-Earth magnetic stir-bar - our 'flea' (Fisherbrand$^{\text{TM}}$ product number 11561953). The cylindrical flea is 24 mm long and 6 mm in diameter, with hemi-spherical ends. The tank is held aloft by two height-adjustable platforms, to give control over $z_{\text{b}}$. The Perspex cylinder is filled with the fluid under investigation, and the tank is filled with a temperature-monitored water bath. The water here serves two purposes: for closer refractive index matching with the fluid under investigation to limit optical distortion of the cylindrical chamber on imaging; and as a heat source/sink with which to control the temperature of the fluid. We control the temperature of the bath by continuously pumping the water through a Grant FH16-D flow heater and a copper coil submerged in an ice bath. This system provides control of the temperature between 0 and 45°C to within $\pm 0.3$°C, and thus control over the fluid viscosity.

In addition to the use of temperature control, we varied viscosity through the use of different solutions, including glycerol (Sigma Aldrich, product no. G9012) - distilled water mixtures, aqueous poly(ethylene glycol) (PEG) solutions ($\text{M}_{\text{w}} = 35,000$ g mol$^{-1}$, Sigma Aldrich, product no. 81310), Castor oil (Sigma Aldrich, product no. 259853) and various types of honey. Glycerol and PEG solutions suffer from different problems when conducting this viscosity-sensitive experiment: glycerol is hygroscopic, so absorbs atmospheric moisture over time, and the solvent in the PEG solution evaporates. To limit these effects, the cylinder was kept sealed using Parafilm at all times except during experiment when more transparent polyethylene film (commonly known as 'cling film' in the UK, or Saran Wrap in the US) was used.

We measured the viscosity of each of our solutions, at a range of temperatures, using a TA Instruments HR-1 Hybrid Rheometer. A secondary problem with polymer solutions is that they are often shear thinning; viscosity decreases with increasing shear rate. For this reason, we chose solutions (polymer concentration by mass $c_0 < 35\%$, and molecular weight $M_{\text{w}} = 35$ kg mol$^{-1}$) that we find to be well approximated as Newtonian under the conditions relevant to our experiments. In the majority of experiments, pure glycerol is the liquid under examination, with $T = 24°$ C, and $\eta = 0.99$ Pa s.

### Waggle characterisation

Here we discuss the method we use to measure the motion of the fles. We position a Casio Exilim camera above (for imaging angular dyynamics) or to the side (for imaging vertical motion) of the chamber and record images between 60 and 480 fps. We use ImageJ software to extract the angular and centroid position of the flea in each video frame. From the side, where optical distortions due to the curved cylinder may be expected, we only measure the centroid position of the flea, which only moves vertically, and so optical distortions will not affect these data. We fit the angular data using a least squares minimization routine in Python, aided by using various analytical methods to extract estimates for the initial input parameters (to which the fitting routine was sensitive) from the raw data, including linear fitting for $\omega_{\text{s}}$ and $\phi$, Fourier transform for $\omega_{\text{w}}$, and mean square calculation for $A$.

### Flea properties

Here we describe our methods for experimentally measuring the properties of the flea relevant to our experiments, and the subsequent forces acting on it; inertia, viscous drag, and magnetic coupling. We measure the moment of inertia of the flea directly using the TA Instruments HR-1 Hybrid Rheometer, by attaching the flea to a rheometer plate with a thin piece of double sided tape. This gave a value of $0.10954 \times 10^{-6}$kgm$^2$.

We measured the magnetic moment of the drive magnet and flea, by using a Kern mass balance (model number ALJ-160 4NM, sensitivity $\pm 0.1$ mg) to measure the weight of the flea as either a second flea, or the drive

magnet, was lowered towards it. Taking care to ensure the centroid positions and dipoles of magnets were well aligned ($\Delta x \approx 0$, $\Delta y \approx 0$ and $\phi \approx 0$), the balance and adjustable platform were level (horizontal to gravity), and the flea's magnetic attraction to the Kern mass balance was negligible (tested by checking the mass read-out is not altered by moving the closer towards or further away from the mass balance), we could then use the vertical component of the dipole-dipole force equation on a magnet, $F = (3\mu_0 m_\mathrm{d} m_\mathrm{f}\cos(\phi)/4\pi z^4)\hat{z}$ to calculate the two magnetic moments. This technique yielded values of $m_\mathrm{d} = 8.4 \pm 0.2$ Am$^2$ and $m_\mathrm{f} = 0.13 \pm 0.1$ Am$^2$.

### Numerical analysis of vertical motion

Our analytic solutions are unable to predict the vertical motion of the flea, and so in this section we describe how we used numerical methods to calculate the behaviour in the $z$ axis. To calculate the mean vertical position with time, we run iterative numerical routines in Python that, using the `odeint` package, numerically solve the coupled equations of motion (1) and (2), with time step of 10 $\mu$s, typically for 10 s. We further add an elastic repulsion at $z = z_\mathrm{b}$ to simulate the effect of the solid base of the container. We define the terminal velocity as $v_\mathrm{t} = mg'/6\pi\eta RJ$, where $m$ is the mass of the flea, $g'$ is the buoyancy corrected gravitational acceleration ($mg' = mg - \rho V g$, where $V$ is the volume of the flea), $R$ is the semi-minor axis of the flea ($R = 3$ mm) and $J$ is a scaling factor for an ellipsoid falling in the direction of its shortest axis, given by

$$J = \frac{\frac{8}{3}(\beta^2 - 1)}{\frac{2\beta^2-3}{\sqrt{\beta^2-1}}\ln\left(\beta + \sqrt{\beta^2-1}\right) + \beta}, \qquad (1)$$

where $\beta = l/R$ [27], and has the value $J = 2.06$ for our flea. The equilibrium, non-rotating, aligned magnet vertical position, $z_0$, is defined as $z_0 = (3\mu_0 m_\mathrm{d} m_\mathrm{f}/4\pi m g')^{\frac{1}{4}}$.

### Fluid flow simulations

In this section we describe our computational simulations of the fluid flows, and subsequent forces acting on an eccentric flea. These simulations are based on an embedded boundary method described previously [19-21] (here we used a 0.25 mm lattice spacing and 0.01 ms time-step), and solved using the projection method [28]. As described in previous work, these simulations assume that the fluid obeys discretized Navier-Stokes equations embedded on a staggered mesh [29], and achieve two-way coupling between the spheres and the fluid using the template model. Here, the flea was modelled as a cylinder, oscillating such that it mimics the motion of the flea, where the parameters matched the waggler experiment as closely as possible, including viscous and inertial forces. This method predicts the fluid flow generated in response to the waggling motion (Fig. 3 c in main article), and the resulant force induced by an eccentric waggle, oscillating 2 mm off-centre (Fig. S1).

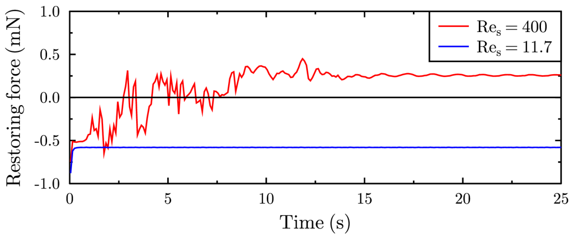


FIG. S1: Plots of the computationally simulated restoring force acting on an eccentrically waggling cylinder, over a 25 s period. Negative values indicate a force in the direction toward the end with the smallest amplitude, which show only for low $\mathrm{Re_s}$ can the eccentric waggle provide steady inward restoring force to maintain levitation stability.

## AUXILLARY EXPERIMENTS

### Wall Effects I. The base of the container

One initial experimental unknown is the extent to which the base and walls of the chamber affect the viscous torque exerted on the flea. The effect of the base is particularly important when the experiment begins as the flea is in contact with the base. Analytic solutions for the increase to viscous drag when a traveling particle is brought close to a parallel wall break down when they are in contact as singularities appear in the equations [30]. Clearly the viscous torque is not infinite when the experiment begins and the flea is spinning on the base of the container, so care is needed to estimate the effect of the wall when predicting the transition frequency to waggling, $\omega_\uparrow$. We attached a bespoke flea-shaped geometry to our TA Instruments HR-1 Rheometer to measure the torque exerted by the fluid as the rod approached the base of the chamber. An initial approximation of the vertical position of the base of the chamber was identified using the rheometer's base-finding function. We then raised the rod's position by 1 mm, and lowered the rod in increments of 10 $\mu$m, performing rheological analysis at each step (vertical resolution 0.2 $\mu$m). At 90 $\mu$m above the initial base position approximation, the rod's motion is not smooth during measurement, indicating that it is coming into contact with the base, and so this is chosen as our 'contact point', where $z = z_\mathrm{base}$. The experiment was then repeated without the rod attached, to take into account the torque exerted by the rest of the geometry. The results indicated a relative increase of $\gamma \approx 3.43$ of the viscous forces when the rod was in 'contact', compared

to when it is 2 cm above the base, where measurements show no continued reduction in drag from increasing the spacing further (*i.e.* the height at which wall effects become negligible).

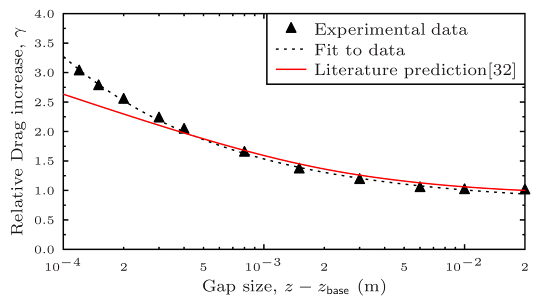


FIG. S2: Plot of measured relative increase to the viscous torque on a flea-shaped brass geometry by the nearby base of the beaker, $\gamma$, against distance from the base of the beaker, $z - z_{\mathrm{base}}$. Dashed line is our fit to the data, which is subsequently used in our numerical calculations of average levitation height. Solid red line is theoretical prediction from Zeng *et. al* [30] for a rod shaped particle moving parallel to a wall, and perpendicular to its longest axis.

In Fig. S2 we have plotted these data against the predictions of Zeng *et al.* [30] for a rod-shaped particle moving parallel to a nearby wall, and perpendicularly to its longest axis, normalising both by the value at 2 cm away from the wall. These plots are in fairly good agreement despite the difference between a rotating and translating geometry. While only a single value of $\gamma = 3.43$ is used to estimate $\omega_{\uparrow}$, a full fit to this experimental curve was used in the viscous forces component of our numerical calculations of the average height of the flea. Additionally, measurements taken with our bespoke flea-shaped rheometer attachment justify the use of the low Reynolds number drag assumption: the ratio of viscous torque to drive speed was constant for all speeds relevant to our experiment.

### Wall Effects II. Stability in large vessels

In some experiments, in which the flea was spun up in large containers (up to 15 times the length of the flea), the transition to stable levitation was not consistent, in the sense that sometimes it jumped up to a stable levitation point, and sometimes it instead jumped outwards to rattle against the walls of the container. In an attempt to quantify this effect, we performed a series of experiments with a chamber within a chamber; an initially small, removable, open-ended cylindrical vessel to prevent the flea being thrown out away from the levitation point (48 mm diameter), within a much larger vessel (360 mm diameter). We find that, with glycerol, when a smaller vessel diameter is initially used to ‘encourage’ the flea into its stable levitation position, increasing the chamber size by removing the smaller diameter cylinder did not disrupt the stability, over any timescale. From this, we conclude that, while a small vessel increases the chances that the flea will end up at the stable levitation position, once there, the size of the vessel has very little effect. This was true for all vessel sizes we tested, with diameters up to 15 times the length of the flea.
